# Supplementary material for: Omni-Line-of-Sight Imaging for Holistic Shape Reconstruction
Source: arXiv:2304.10780 source file (2023-04-21)
Supplement: Supplementary file 1 [file 6_supp.tex]

% {\center \huge Supplementary materials}
\appendix

\setcounter{figure}{0}

\begin{figure*}[t]
    \centering
    \includegraphics[width=0.8\textwidth]{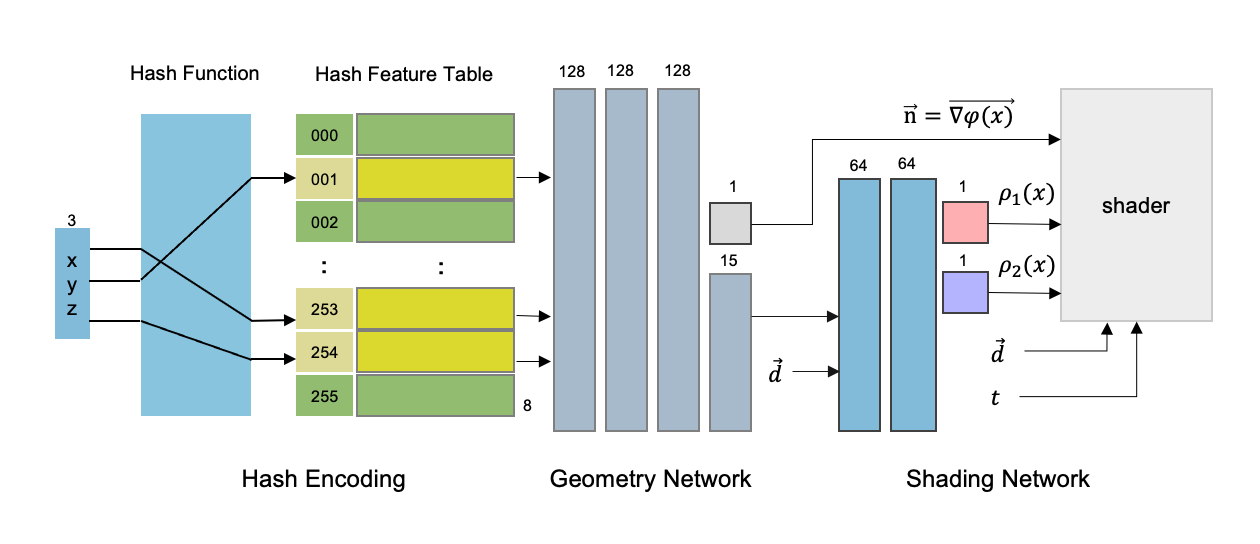}
    \caption{Network architecture. Our network is implemented as a shallow MLP augmented with Hash Encoding~\cite{mueller2022instant}. It takes as input a coordinate and view direction to predict both a level set and a directional albedo. Thanks to our level-set representation, we can derive surface normal from the level set for computing shading following the light transport equation.}
    \label{fig:network_arch}
\end{figure*}

\section*{A. Volumetric transient rendering} 
Our formulation is a transient volumetric rendering of neural surfaces. We first review volumetric rendering with Transient cameras. Volumetric transient rendering has been explored in To\"RF~\cite{attal2021torf} and NeTF~\cite{shen2021non},  whose procedure is to apply rays tracing through the volume and integrate the radiance along the geometry of light transport. In NeRF~\cite{mildenhall2020nerf}, the radiance along the ray observed by a camera defines as 
\begin{equation}
    L(\measurepoint, \omega_o) = \int_{0}^{t}\transmittance(\measurepoint, \point)\density(\point)L_s(\point, \omega_o)dt
\end{equation}
where 
\begin{equation}
\transmittance(\measurepoint, \point) = \exp{(-\int_{0}^{t}\density(\measurepoint-\omega_os)ds)}
\end{equation}
is the transmittance for light propagating from position $\point$ to $\measurepoint$, where $\omega_o = \widehat{\point\measurepoint}$.
$L_s(\point, \omega_o)$ is the outgoing radiance at $\point$, typically referring to colors in NeRF. However, the volume rendering equation in
NeRF is essentially a self-emission model for a conventional camera. For a ToF-based camera, two changes should be made~\cite{attal2021torf}. First, the $L_s(\x, \omega_i)$ should respond to different light sources as ToF cameras use an active light source to illuminate the scene. Second,  we should impose a path length importance function into the integral as ToF cameras capture radiance according to the time of flight $\timeofflight$. Therefore, 
the transient rendering equation can be expressed as 
\begin{equation}
    L_\text{ToF}(\measurepoint, t, \omega_o) = \int_{0}^{t}
    H(\measurepoint, \point)(\|\point-\measurepoint\|)\transmittance(\measurepoint, \point)\density(\point)L_s(\point, \omega_o)dt
    \label{eq:tof}
\end{equation}
where the function $H(\measurepoint, \point)$ is a weight of the contribution of a light path of length $d$. Typically, SPAD camera uses $W_\timeofflight(d) = \delta(d - \frac{1}{2}\timeofflight c)$. In the next, we derive $L_s(\point, \omega_o)$ for both LOS and NLOS by ray tracing the light source. 
\subsection*{A.1. LOS Rendering}
Under the ideal LOS setting, the ToF camera can observe radiance directly from the object, which is only illuminated by the point light source collocated at the camera position without ambient light. With this assumption, we can model the surface radiance as a function of a light source, 
\begin{equation}
    L_s(\point, \omega_o) 
    = \underset{\Omega}{\int}{\albedo(\point, \omega_i, \omega_o)}(\omega_i \cdot  \normal(\point))L_i(\point, \omega_i)
    d\omega_i 
    \label{eq:surface_radiance}
\end{equation}
where $L(\point, \omega_i)$ is the incident illumination from direction $\omega_i\in\Omega$, $\Omega$ is the unit hemisphere centered around $\normal(\point)$ containing all possible values for all $\omega_i$ where $(\omega_{i}\cdot \normal > 0)$, and $\albedo(\point, \omega_i, \omega_o)$ is the BRDF function. 
As only a point light source collocated at the camera position, each surface area is only illuminated from one direction. Following \cite{shen2021non} and \cite{attal2021torf}, we ignore the forward scattering of the incident radiance as our scene consists of nearly solid surfaces. Therefore, 
\begin{equation}
    L_{i}(\point, \omega_i) = \frac{I}{\|\point-\measurepoint\|^2}\delta(\widehat{\point\measurepoint}-\omega_i)\transmittance(\measurepoint, \point)
    \label{eq:light_radiance}
\end{equation}
where the scalar $I$ represent the emitted radiant intensity and $1/\|\point-\measurepoint\|^2$ is the inverse square light fall-off. By substituting Eq.~\ref{eq:light_radiance} and Eq.~\ref{eq:surface_radiance} into Eq.~\ref{eq:tof}, we can derive 
\begin{equation}
\begin{aligned}
    L_\text{ToF}(\measurepoint, \timeofflight, \omega_o) = \int_{0}^{t}\delta(\|\measurepoint-\point\|-\frac{1}{2}\timeofflight c) \\
    I\frac{(\normal\cdot\widehat{\point\measurepoint})}{\|\measurepoint-\point\|^2}\transmittance^2(\measurepoint, \point)\density(\point)
    \rho(\point, \widehat{\point\measurepoint}, \widehat{\point\measurepoint})dt \eqstop
\end{aligned}
\end{equation}

By rotating the transient camera, 
we acquire transient measurement forming a frustum. For clarity, we can define the virtual sensor spot $\point$ on the image plane by
 reparameterizing $\spadposition = \measurepoint + d \delta$ with and $d=-\omega_o$ and $\delta$ being a small constant. By ignoring the constant terms, we represent our LOS rendering equation as 
 \begin{equation}
\begin{aligned}
	\losmeas(\spadposition, \timeofflight) =  \int_{\hat{\Omega}}\delta(\| \spadposition - \point \| - \frac{1}{2}\timeofflight c) 
 \\
 \frac{(\normal\cdot \widehat{\point\spadposition})
 }{\|\point-\spadposition\|^2}
 \transmittance^2(\spadposition, \point)
 \density(\point)\albedo(\point, \direction)d\point \eqstop
 \end{aligned}
\end{equation}
where we denote the $\hat{\Omega}$ to represent the ray. 

\subsection*{A.2. NLOS Rendering}
We now derive the NLOS rendering equation. 
Whereas under the LOS setting, we observe radiance from the object directly with ToF cameras, under the NLOS setting, we only observe radiance from the relay wall. We should recursively trace the ray to the surface and light source to recover the hidden object occluded from direct view. We assume that are up to three bounce, \ie, scattering from relay wall $\point_w$ to hidden surface $\point$ and back to the relay wall $\point_w$. We assume that the relay wall is purely diffuse, \ie, light scattering equally in all directions. Notice that the diffuse wall receives photons bounced from the surface. For clarity,  we denote the ray direction from $\point_1$ to $\point_2$ as $\widehat{\point_1\point_2}$. 
With these assumptions, we can formulate the radiance at $\wallposition$ at the diffuse wall as 
\begin{equation}
\begin{aligned}
    L_\text{ToF}(\measurepoint, \widehat{\point_w\measurepoint}, t) = \underset{\Omega}{\int}H(\measurepoint, \point)
    \rho_{w}L_w(\point_w, \widehat{\point_w\point})(\normal_w\cdot\widehat{\point_w\point})d{s(\point)} \\
    = \underset{\Omega}{\int}\rho_{w}L_w(\wallposition, \widehat{\wallposition\point})(\normal_w\cdot\widehat{\point_w\point})\frac{(\widehat{\point\wallposition}\cdot \normal)}{\|\point-\wallposition\|^2}
    d{\widehat{\point_w\point}} 
\end{aligned}
\label{eq:wall_obvervation}
\end{equation}
where $\rho_{w}$ is a constant. 
Following Eq.~\ref{eq:surface_radiance}, we can trace radiance from the object to the wall by 
\begin{equation}
    L_w(\wallposition, \widehat{\wallposition\point}) = \int_{L} \transmittance(\wallposition, \point)\density(\point)L_s({\point, \widehat{\point\wallposition}})d\point \eqcomma
    \label{eq:surf_to_wall}
\end{equation} where $L$ is a ray trace from $\wallposition$ to $\point$. 
Following the assumption \cite{attal2021torf} we ignore the forward scattering from light to the surface, 
\begin{equation}
\begin{aligned}
    L_s(\point, \widehat{\point\wallposition}) = \underset{\Omega}{\int}{\albedo(\point, \omega_i, \omega_o)}
    (\normal_w\cdot\widehat{\point_w\point})L_i(\point, \widehat{\point_w\point})d{\widehat{\point_w\point}} 
    \label{eq:wall_to_surf}
\end{aligned}
\end{equation}
The incident radiance is constant as light scatters equally from the wall position. Under the NLOS setting, the surface is illuminated by a small patch on the relay wall instead of a point source. Plus, we only illuminate only single spot, so each surface is illuminated from only one direction; therefore, 
\begin{equation}
    L_{i}(\point, \widehat{\point\wallposition}) = \frac{I(\normal_w\cdot\widehat(\wallposition\point)}{\|\point-\measurepoint\|^2}\delta(\widehat{\point\measurepoint}-\omega_i)\transmittance(\wallposition, \point)
    \label{eq:wall_illumination}
\end{equation}

By tracing the ray from sensor to the laser via Eq.~\ref{eq:wall_obvervation}, Eq.~\ref{eq:surf_to_wall}, Eq.~\ref{eq:wall_to_surf} and Eq.~\ref{eq:wall_illumination}, 
we obtain 
\begin{equation}
\begin{aligned}
    L_\text{ToF}(\measurepoint, \widehat{\wallposition\point}) = \underset{\Omega\times L}
{\int}H(\measurepoint, \point)
% fall off 
\frac{(\normal\cdot\widehat{\point\wallposition})^2(\normal_{w}\cdot\widehat{\wallposition\point})^2 
}{\|\point-\wallposition\|^4}  \\
\transmittance(\wallposition, \point)^2\rho(\point, \widehat{\point\wallposition},\widehat{\point\wallposition})
\density(\point)d\point
\end{aligned}
\end{equation}
where we ignore all constants for clarity. We then can incorporate the path length weighting function to convert it into a transient measurement parameterize the wall position
\small{
\begin{multline}
	\nlosmeas(\wallposition, t) = \underset{\hat{\Omega}}{\int}  \delta(\| \wallposition - \point  \|-\frac{ct}{2})
\frac{(\normal\cdot\widehat{\point\wallposition})^2(\normal_{w}\cdot\widehat{\wallposition\point})^2
}{\|\point-\wallposition\|^4}
\\
 \transmittance^2(\wallposition, \point) \density(\point) \albedo(\point, \direction)  d\point\eqstop
\end{multline}
}
where $\hat{\Omega}$ is a 3D sampling space.

\section*{B. Additional implementation details}
\subsection*{B.1 Discrete forward model}
We detail our network architecture in Fig.~\ref{fig:network_arch}. 
Here we describe our implementation of the NLOS forward model, where the LOS forward model can be implemented easily by only shooting one ray. Recall that under a confocal setting, the full image formation model can be expressed as:
\begin{equation}
\small
\begin{aligned}
\nlosmeas(\wallposition, t) = \underset{\hat{\Omega}}{\int}  \delta(\| \wallposition - \point  \|-\frac{ct}{2})\\ 
\underbrace{\frac{(\normal\cdot\widehat{\point\wallposition})^2(\normal_{w}\cdot\widehat{\wallposition\point})^2
}{\|\point-\wallposition\|^4}
\albedo(\point, \direction)}_{\text{shading}~f(\point)}
\underbrace{
\transmittance^2(\wallposition, \point) \density(\point)
}_{\text{weight}~w(\point)}d\point\eqstop
\end{aligned}
\end{equation}
We denote $f(\point)\ge 0$ as a shading function, which can be evaluated directly with a single position. We denote the sample weight as $w(\point)$. Neural transient rendering then is to evaluate both $f(\point)$ and $w(\point)$ and summation. Here we describe our discrete forward model. 
We use spherical coordinates to parameterize the $\point=(x,y,z)$ with $(\theta, \phi, r)$ with $\wallposition=(x_0, y_0, z_0)$ being the origin so that 
\begin{equation}
\left\{
\begin{aligned}
x &= r\cos\theta\cos\phi + x_0 \\
y &= r\cos\theta\sin\phi + y_0 \\
z &= r \sin\theta + z_0 \\
\hat{r} &= tc / 2
\end{aligned}
\right.
\end{equation}

Therefore, we rewrite the forward model as 
\begin{equation}
\small
\begin{aligned}
    \nlosmeas(\wallposition, t) = \iiint\delta(r-\hat{r})f(\point(r, \theta, \phi))\\ w(\point(r,\theta, \phi)) 
    1/r^2 \sin\theta d\theta\phi \\
    = \iint w(\point(\hat{r},\theta, \phi))f(\point(\hat{r},\theta, \phi))
    1/\hat{r}^2 \sin\theta d\theta\phi\eqstop
\end{aligned}
\end{equation}
where 
\small{
\begin{align}
w(\point(\hat{r}, \theta, \phi)) = \transmittance^2(\point(\hat{r}, \theta, \phi))\sigma(\point(\hat{r},\theta, \phi)) \\
\transmittance(x(\hat{r},\theta, \phi)) = \exp(-\int_{r}^{\hat{r}}\density(\point({r},\theta,\phi)) dr) \eqstop
\end{align}
}

We then discretize the model following~\cite{shen2021non}: 
\begin{equation}
    \nlosmeas(\wallposition, t) = \sum_{i}\sum_{j}
    w(\hat{r}, \theta_i, \phi_j) 
    f({r_k, \theta_i, \phi_j})
    \sin\theta_i / 
\hat{r}^2\Delta\theta_i\Delta\phi_i
\end{equation}
To evaluate $w(r, \theta, \phi)$, we need to compute transmittance along the ray. We omit $\theta$ and $\phi$ for clarity 
\begin{equation}
\transmittance(r) = \exp(-\sum_{k}\density(r_k))\Delta r_k)
\end{equation}

\begin{figure}[t]
    \centering
    \includegraphics[width=0.8\columnwidth]{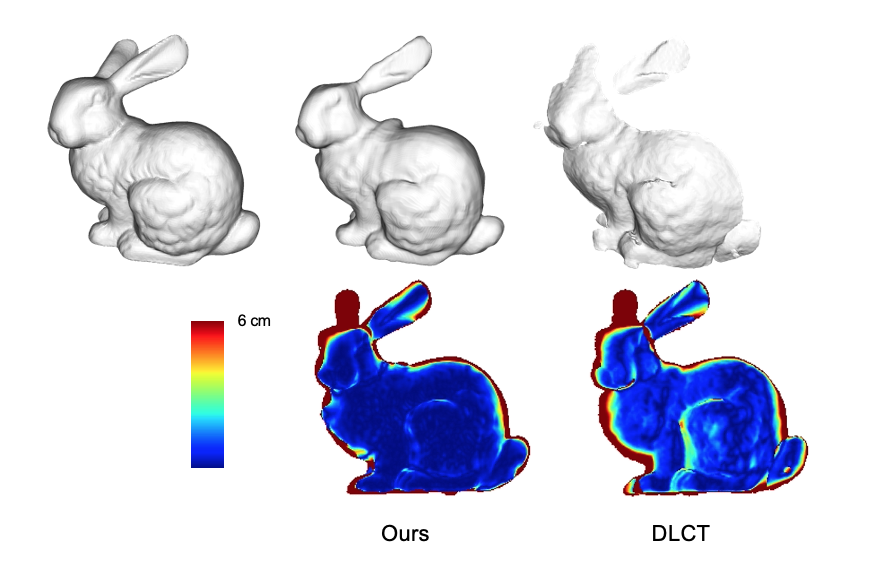}
    \caption{Comparison of our method to DLCT on single wall NLOS reconstruction. We show the extracted mesh as well as the depth error map. Our method recovers the bunny accurately in the boundary, such as the right ear.}
    \label{fig:single_wall_comp}
\end{figure}

\paragraph{Shading with normal}. Notice that our formulation incorporates surface normal to compute $f(\point)$. The normal is the gradient of the level set 
\begin{equation}
    \normal = \frac{\nabla(\levelset(\point))}{\|\nabla(\levelset(\point)) \|+\epsilon}
\end{equation}
computed by auto differentiation. Notice that some voxels face backward. To output a valid $f(\point)$, 
we truncate it by $\max(f(\point), 0)$. 
\par

\subsection*{B.2 Noise prediction}
Our method assumes our scene consists only of opaque surfaces. It is crucial to model the noise for real captured data as our method will treat noises incorrectly as surfaces. To offset the noise predicted by our method, we model a noise field conditioning of a location and an optimizable embedding to account for different lighting. The predicted transient from the physically-based modeling is then offset by the predicted noise transient. We implement the noise fields as a two-layer MLP with $64$ hidden dim that takes as input the hash embedding and an optimizable $64$-dim latent embedding indexed by the sensor position to output a noise value. We then `render' the noise into transient according to  Eq.~15. 

\section*{C. Additional results}

\subsection*{C.1 Single Wall NLOS reconstruction}
To evaluate the performance of our surface reconstruction method for hidden objects, we adopt a simulated confocal measurement with third bounce reflections from a hidden bunny from \cite{galindo19-NLOSDataset}. The measurements acquired correspond to $256 \times 256$ points uniformly sampled over a $1m\times 1m$ area and $512$ time bins with a temporal resolution of $4$ ps per bin. Fig.~\ref{fig:single_wall_comp} shows our method's reconstruction results and DLCT's depth error map. The MAE/RMSE is 1.18/2.29~cm and 1.57/2.42~cm for ours and DLCT, respectively. Our method is moderately better than DLCT. This demonstrates our NLOS rendering and learning procedure is more accurate. Our method can handle various scenes, including real data and specular scenes. we include more results in Fig.~\ref{fig:single_wall_more}. 

\begin{figure}[t]
    \centering
\includegraphics[width=0.8\columnwidth]{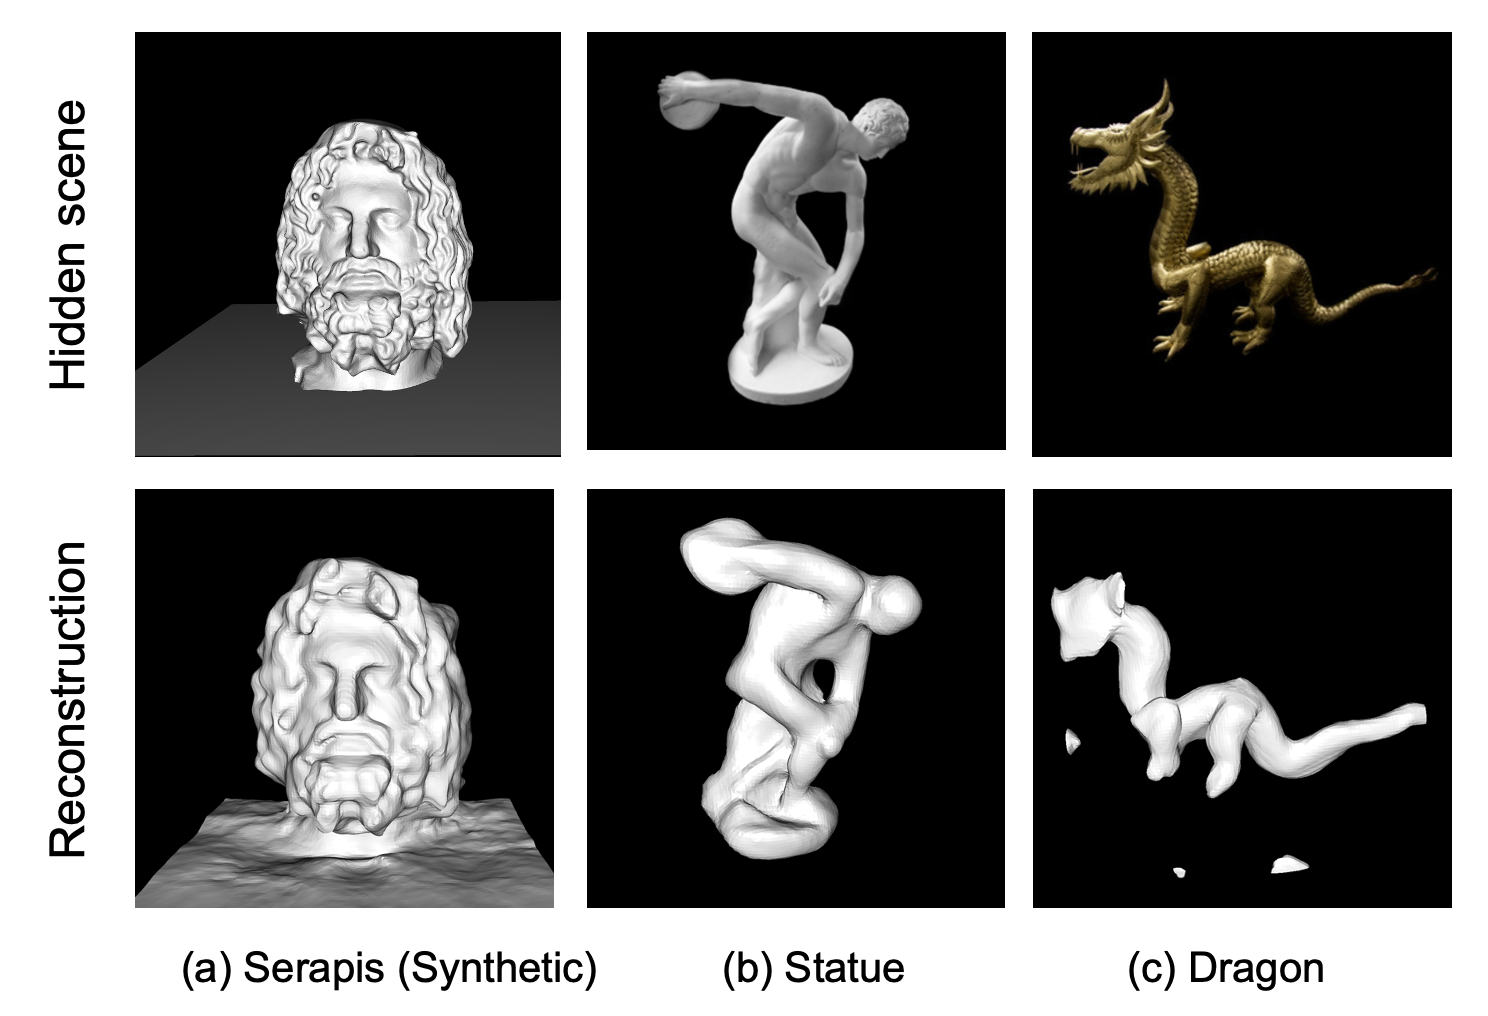}
    \caption{More results of single wall NLOS recovery. (a) is a synthetic data will floor, while (b) is real captured data with diffuse materials, and (c) is real captured data with specular materials. 
    Our method reasonably recovers surfaces for various scenes. The synthetic Serapis is from \cite{}, and the real data is from \cite{2019FK}.}
    \label{fig:single_wall_more}
\end{figure}

\begin{figure*}[t]
    \centering
    \includegraphics[width=\textwidth]{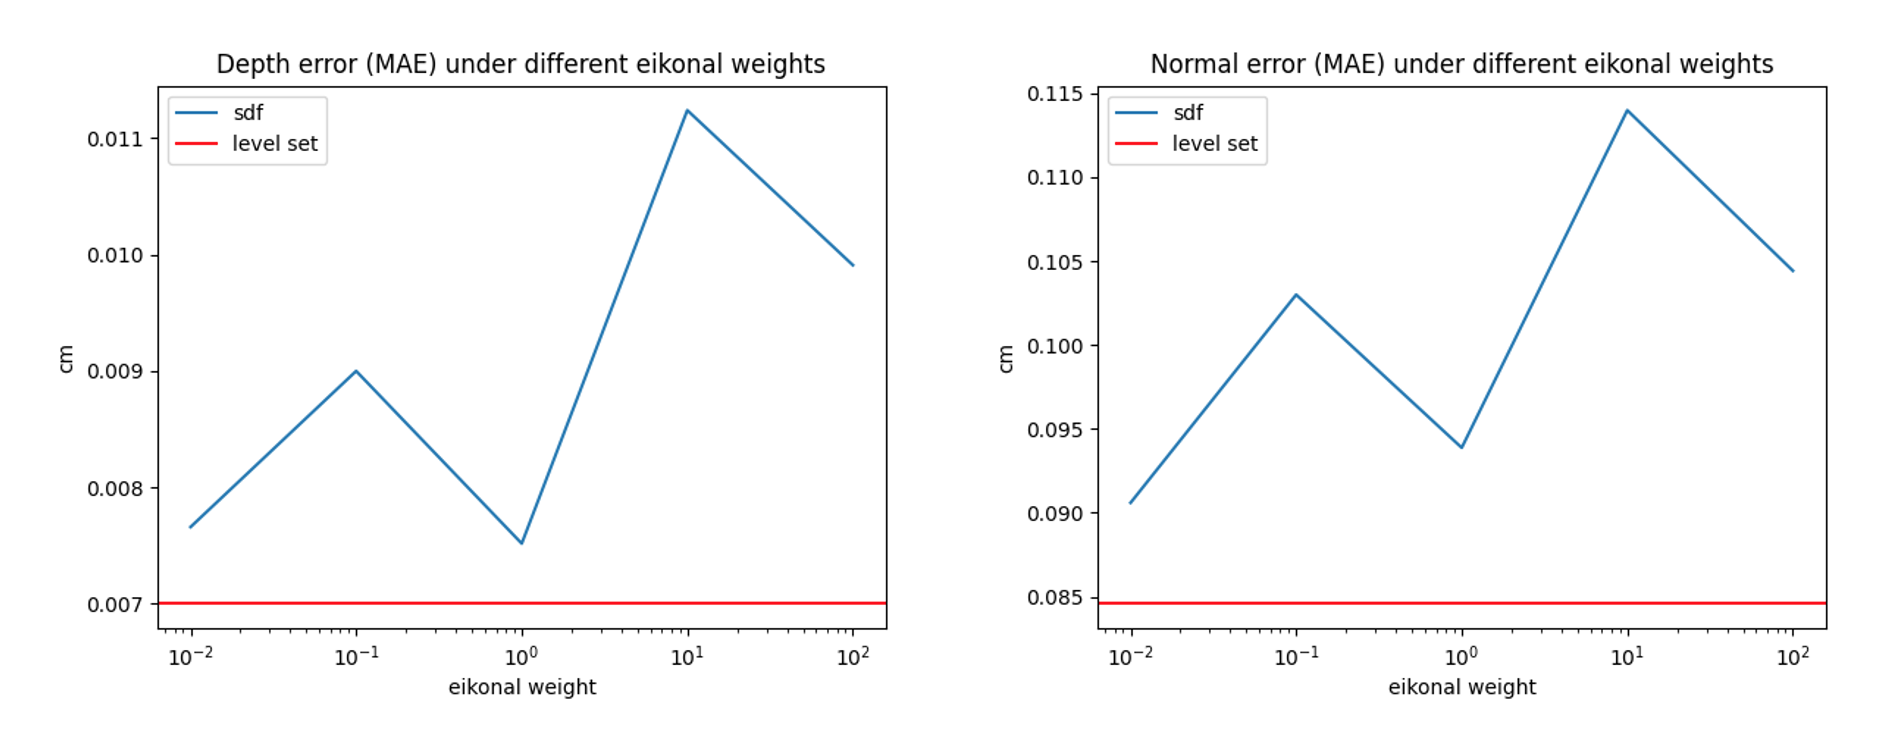}
    \caption{Level set V.S. SDF. 
    A level set representation does not require the $\|\nabla\levelset(\point)\| = 1$,  with more flexibility to recover the scene. }
    \label{fig:sdf}
\end{figure*}

\subsection*{C.2 Level set V.S. SDF}
SDF neccessatates eikonal loss to ensure $\|\nabla\levelset(\point)\| = 1$. Previous methods \cite{wang2021neus, yariv2021volume} assume that the magnitudes of the gradient are $1$ and ensure this through regularization, while our method incorporates the magnitudes of gradient on the forward model. Although tuning the weight of eikonal loss would achieve better results, \eg, smoother surface, 
we empirically find a level set representation without eikonal loss is sufficient under our scenarios. To validate this, we modify our forward model by letting $\nabla\levelset=\normal=\frac{\nabla\levelset}{\|\nabla\levelset\|}$ following \cite{wang2021neus}, and impose eikonal regularizer\cite{tsai2017geometry} with various weights. We conduct experiments on a Stanford bunny with 10$k$ iterations and keep other parameters the same. For SDF, we additionally uniformly sample $100k$ points for eikonal regularization. 
Fig.\ref{fig:sdf}~ shows the results. 

\section*{D. Holistic reconstruction results}
We include more cases and compared methods in Fig.~\ref{fig:gallery}. 
\begin{figure*}[t]
    \centering
\includegraphics[width=\textwidth]{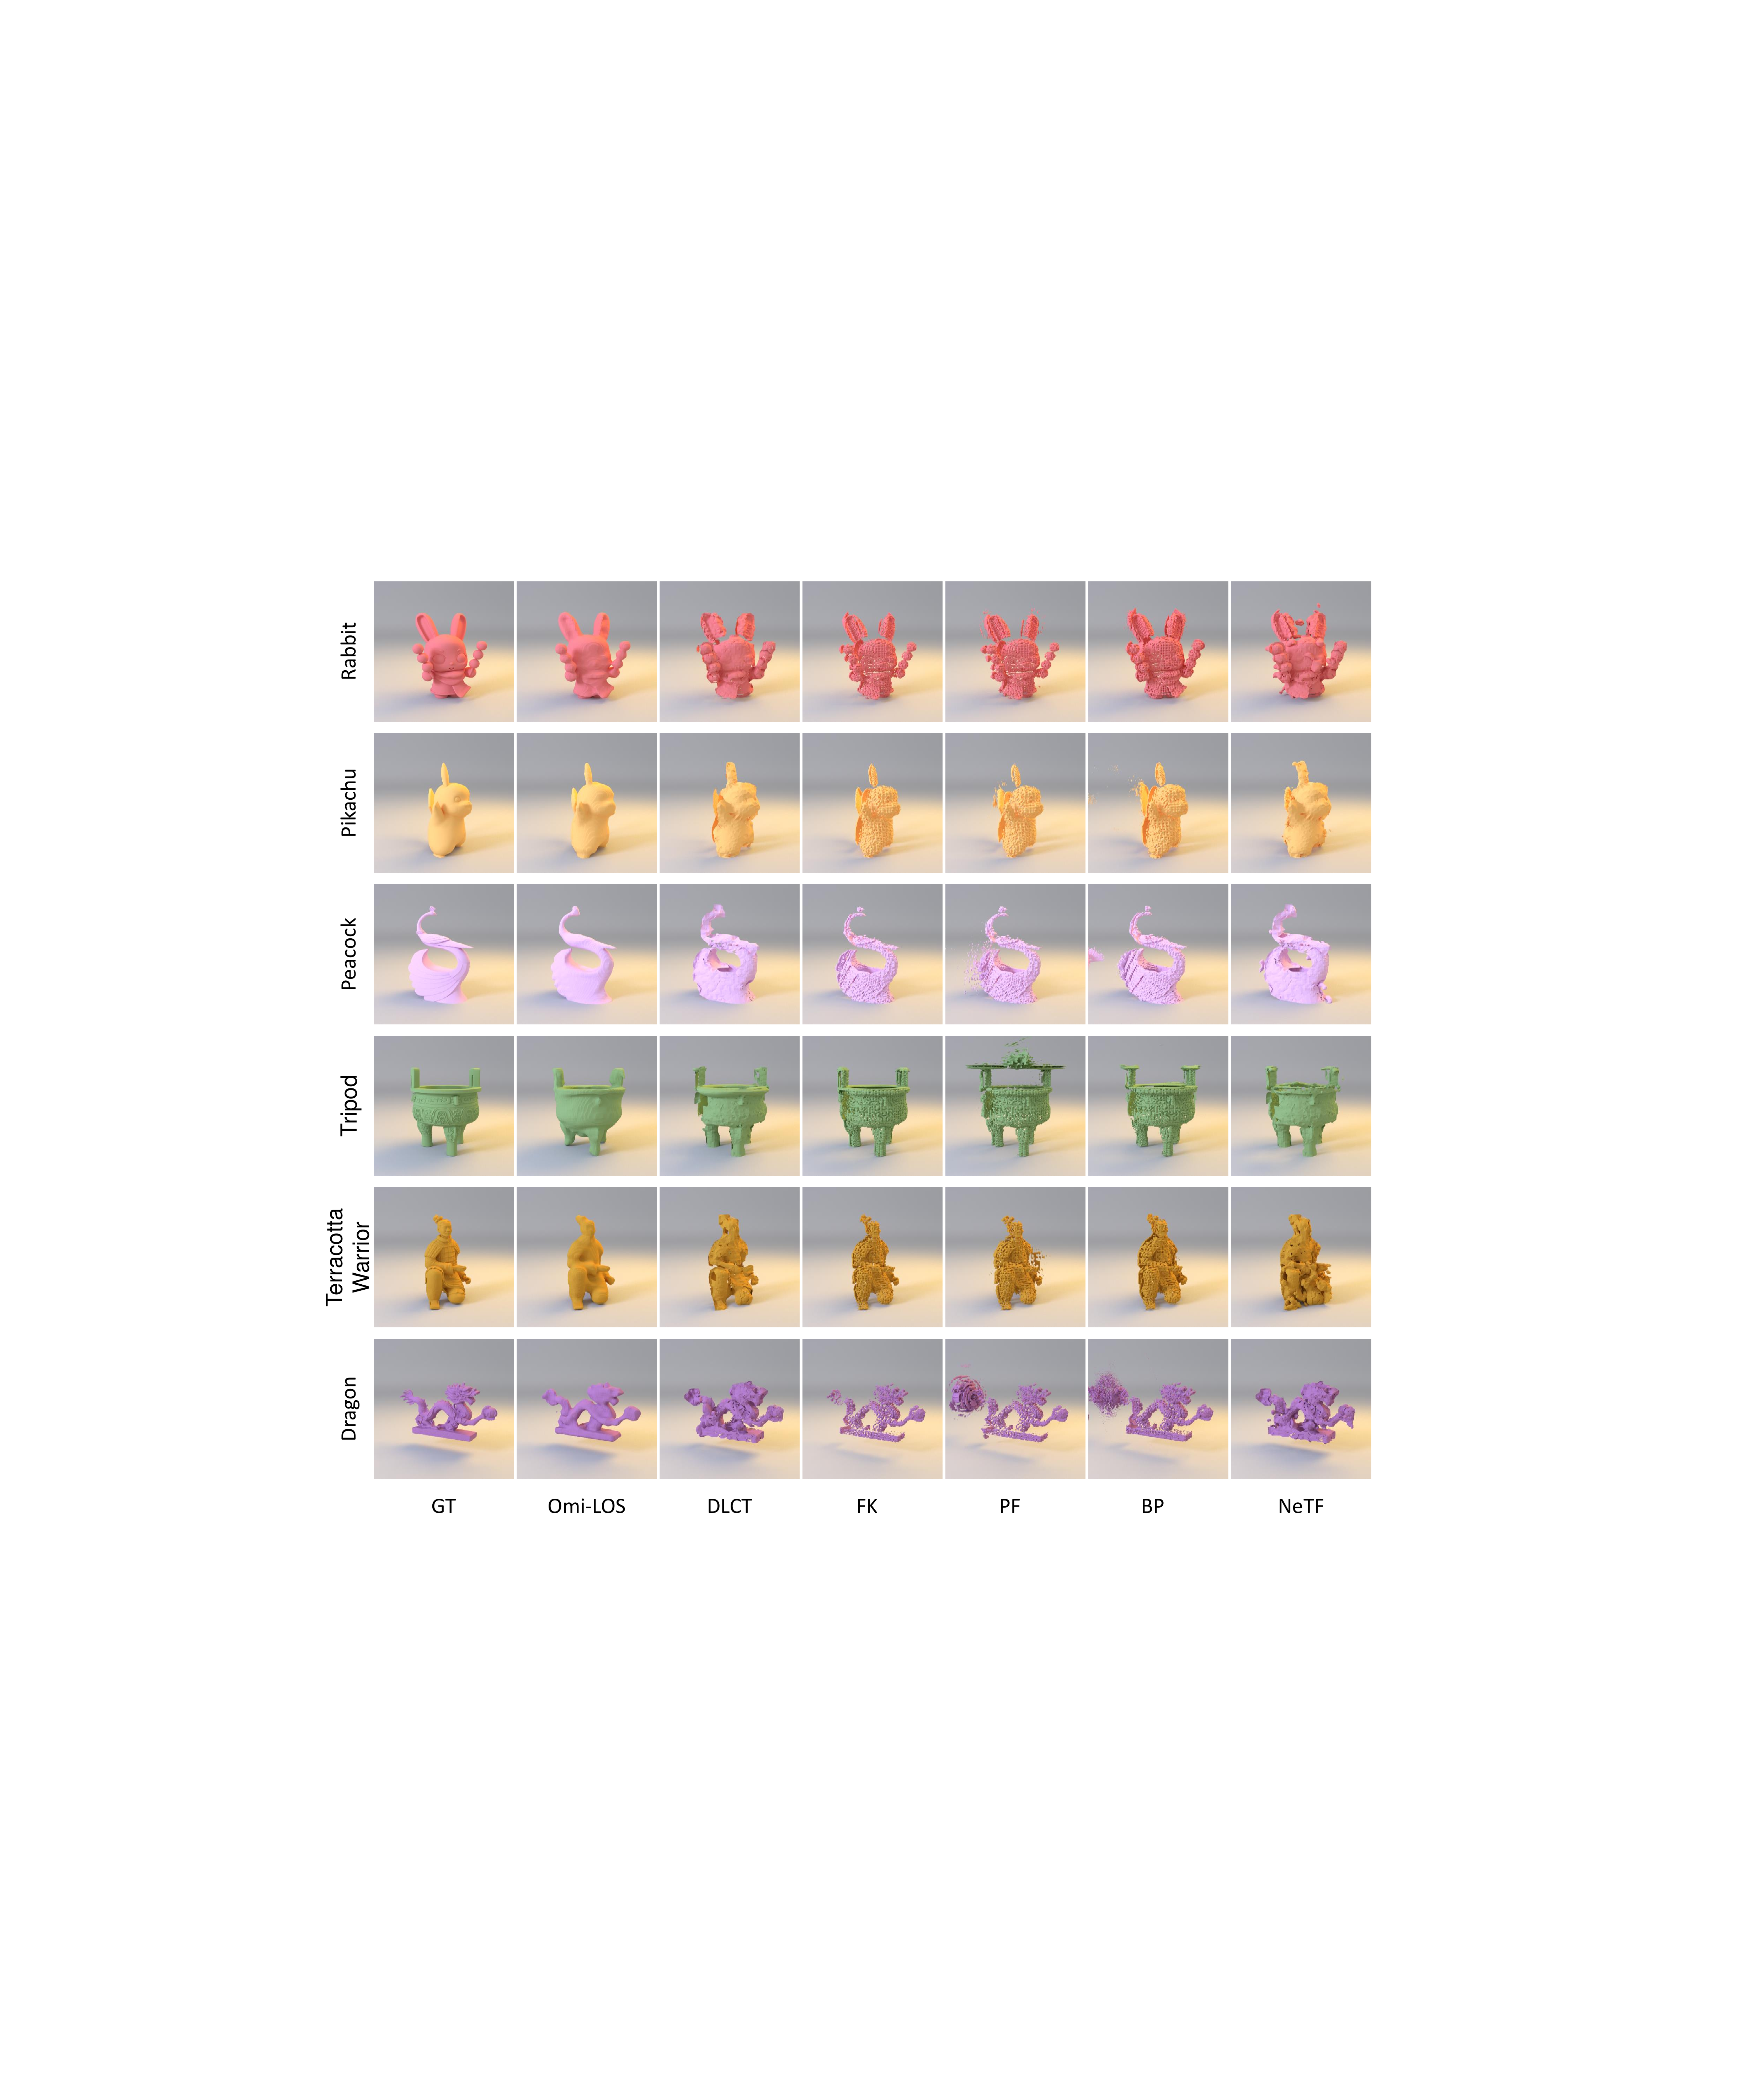}
    \caption{More results of holistic shape reconstruction.}
    \label{fig:gallery}
\end{figure*}
